# Supplementary material for: Composition Dependent Instabilities in Mixtures With Many Components
Source: arXiv:2211.04170 source file (2022-11-08)
Supplement: Supplementary file 1 [file supplementalMat.pdf]

# Supplemental Material for Composition Dependent Instabilities in Mixtures With Many Components

Filipe C. Thewes,[1] Matthias Krüger,[1] and Peter Sollich[1,2]
[1] Institut für Theoretische Physik, Georg-August-Universität Göttingen, 37077 Göttingen, Germany
[2] King's College London, Department of Mathematics, Strand, London WC2R 2LS, U.K.

## 1. SPINODAL EQUATION

We discuss here how to derive the spinodal equation (3) in the main text using free probability theory.

We first introduce some useful transforms from free probability theory [1, 2] and work in the limit of a large number of components, i.e. $M \to \infty$. The Stieltjes transform of a matrix $\boldsymbol{X}$ is defined as

$$G_X(\lambda) = \int \frac{p(x)}{\lambda - x} dx \tag{S1}$$

where $p(x)$ is the distribution of eigenvalues of $\boldsymbol{X}$. The transform (S1) is the $M \to \infty$ version of the normalized trace of the resolvent matrix $(\lambda \boldsymbol{I} - \boldsymbol{X})^{-1}$. If we denote by $K_X(\gamma)$ the functional inverse of $G_X(\lambda)$, i.e. $K_X(G_X(\lambda)) = \lambda$ then, under the assumption of freeness, the sum of two large random matrices obeys the free sum rule $K_{X+Y}(\gamma) = K_X(\gamma) + K_Y(\gamma) - \frac{1}{\gamma}$. Two matrices are said to be free if their eigenvectors are randomly rotated with respect to each other.

The definition (S1) implies that all eigenvalues $x$ of the matrices being considered must be $O(1)$ when applying free probability theory. We therefore switch from the original stability matrix $\boldsymbol{H} = \boldsymbol{R}_1 + \boldsymbol{D} + s\boldsymbol{\eta}$, which has eigenvalues of $O(M)$, to $\tilde{\boldsymbol{H}} = \boldsymbol{H}/M = \tilde{\boldsymbol{R}}_1 + \tilde{\boldsymbol{D}} + \tilde{s}\tilde{\boldsymbol{\eta}}$ where $\tilde{\boldsymbol{R}}_1 = \boldsymbol{R}_1/M$, $\tilde{\boldsymbol{D}} = \tilde{\boldsymbol{D}}/M$, while for the last term $\tilde{s} = M^{-1/2}s$ and $\tilde{\boldsymbol{\eta}} = M^{-1/2}\boldsymbol{\eta}$ is a symmetric Wigner matrix with entries of standard deviation $M^{-1/2}$, which again has $O(1)$ eigenvalues. Such a Wigner matrix has a rotationally invariant distribution and thus randomly oriented eigenvectors. Rigorously, this requires that the variance of the diagonal entries of $\tilde{\boldsymbol{\eta}}$ should be twice as large as that of the off-diagonal ones but we ignore this as the effects should become irrelevant in the limit $M \to \infty$ [3]. Explicitly, a Wigner matrix $\tilde{s}\tilde{\boldsymbol{\eta}}$ has [1] $K_{\tilde{s}\tilde{\eta}}(\gamma) = \tilde{s}^2\gamma + 1/\gamma$ and due its randomly oriented eigenvectors is free relative to any fixed or random matrix $\tilde{\boldsymbol{X}}$, so that

$$K_{\tilde{X}+\tilde{s}\tilde{\eta}}(\gamma) = K_{\tilde{X}}(\gamma) + \tilde{s}^2\gamma. \tag{S2}$$

It will be useful to express this free sum rule in the form of a Pastur relation [4] by replacing $\gamma$ by $G_{\tilde{X}+\tilde{s}\tilde{\eta}}(\lambda)$, namely

$$G_{\tilde{X}+\tilde{s}\tilde{\eta}}(\lambda) = G_{\tilde{X}}\left(\lambda - \tilde{s}^2 G_{\tilde{X}+\tilde{s}\tilde{\eta}}(\lambda)\right). \tag{S3}$$

In what follows, we also make use of the moment generating function

$$\psi_{\tilde{X}}(\lambda) = \int \frac{p(x)\lambda x}{1 - \lambda x} dx = \lambda\langle x\rangle + \lambda^2\langle x^2\rangle + \cdots. \tag{S4}$$

To find the spinodal equation we need to find the spectrum of $\tilde{\boldsymbol{H}}$ and in particular, determine when its lowest eigenvalue becomes zero. As discussed in the main text, due to the interlacing properties of eigenvalues [5], in the limit of $M \to \infty$ the spectrum of $\tilde{\boldsymbol{H}} = \tilde{\boldsymbol{R}}_1 + \tilde{\boldsymbol{D}} + \tilde{s}\tilde{\boldsymbol{\eta}}$ is the same as the spectrum of $\tilde{\boldsymbol{D}} + \tilde{s}\tilde{\boldsymbol{\eta}}$ except that the rank one perturbation $\tilde{\boldsymbol{R}}_1$ may give rise to a single outlier. We therefore proceed by obtaining the spinodal equation separately in the outlier and bulk regimes.

### I. Outlier Regime

Let $\theta$ be the single non-zero eigenvalue of a rank one matrix $\tilde{\boldsymbol{R}}_1$. In [5] the authors obtained the location of the outlier eigenvalue of $\tilde{\boldsymbol{R}}_1 + \tilde{\boldsymbol{X}}$, and a condition for this eigenvalue to be an actual outlier, for a generic large random matrix $\tilde{\boldsymbol{X}}$. We briefly review the outline of their proof.

First, without loss of generality, one can assume that, after an appropriate basis change, $\tilde{\boldsymbol{X}}$ is diagonal and $\tilde{\boldsymbol{R}}_1 = \theta \boldsymbol{v}\boldsymbol{v}^\mathsf{T}$ with $\boldsymbol{v}$ being a unit vector such that $\boldsymbol{v}^\mathsf{T}\boldsymbol{v} = 1$. Below in Sec. 4 we provide more details on the distribution

of $\boldsymbol{v}$ but for now we assume it is random, i.e. uniformly distributed over the unit sphere. The eigenvalues $\lambda$ of $\tilde{\boldsymbol{R}}_1+\tilde{\boldsymbol{X}}$ obey

$$\begin{aligned}\det(\lambda \boldsymbol{I}-(\tilde{\boldsymbol{X}}+\tilde{\boldsymbol{R}}_1))\\ =\det(\lambda \boldsymbol{I}-\tilde{\boldsymbol{X}})\det(\boldsymbol{I}-(\lambda \boldsymbol{I}-\tilde{\boldsymbol{X}})^{-1}\tilde{\boldsymbol{R}}_1)=0,\end{aligned}$$

thus showing that $\lambda$ is an eigenvalue of $\tilde{\boldsymbol{X}}+\tilde{\boldsymbol{R}}_1$, but not of $\tilde{\boldsymbol{X}}$, only if 1 is an eigenvalue of $(\lambda \boldsymbol{I}-\tilde{\boldsymbol{X}})^{-1}\tilde{\boldsymbol{R}}_1$. Since this matrix is of rank one, this eigenvalue condition reduces to

$$\theta \boldsymbol{v}^{\mathsf{T}}(\lambda \boldsymbol{I}-\tilde{\boldsymbol{X}})^{-1}\boldsymbol{v}=1. \tag{S5}$$

Now, on average, the distribution of $\boldsymbol{v}$ results in $|v_i|\approx M^{-1/2}$ with random signs, leading to

$$G_{\tilde{X}}(\lambda)=\theta^{-1}, \tag{S6}$$

where we assume $G_{\tilde{X}}$ to be self-averaging such that for large $M$ the average is also the typical value and fluctuations around this are small. (This can be shown by explicit calculation for a uniform distribution of $\boldsymbol{v}$ on the unit sphere, subject to appropriate conditions on the spectrum of $\tilde{\boldsymbol{X}}$.) Applying the inverse transform $K_{\tilde{X}}$ to both sides of Eq. (S6) gives

$$\lambda=K_{\tilde{X}}(\theta^{-1}). \tag{S7}$$

We can now set specifically $\tilde{\boldsymbol{X}}=\tilde{\boldsymbol{D}}+\tilde{s}\tilde{\boldsymbol{\eta}}$ and apply the free sum rule (S2) to (S7), with $\gamma$ and $\tilde{\boldsymbol{X}}$ in (S2) replaced by $\theta^{-1}$ and $\tilde{\boldsymbol{D}}$, respectively. Together with the spinodal condition $\lambda_{\min}=0$ this gives $0=K_{\tilde{D}+\tilde{s}\tilde{\eta}}(\theta^{-1})=K_{\tilde{D}}(\theta^{-1})+\tilde{s}^2\theta^{-1}$ or, after applying $G_{\tilde{D}}(\cdot)$,

$$\theta^{-1}=G_{\tilde{D}}(-\tilde{s}^2\theta^{-1}). \tag{S8}$$

Now, since $\tilde{\boldsymbol{D}}$ is diagonal its eigenvalues are simply the diagonal entries, which from (2) in the main text are $T/(M\bar{\rho}y_\alpha)=T/(\rho y_\alpha)$. We can then rewrite $G_{\tilde{D}}(\lambda)$ as $-\psi_y(\rho\lambda/T)/\lambda$ to obtain

$$\psi_y(-\rho\tilde{s}^2\theta^{-1}/T)=\tilde{s}^2\theta^{-2} \tag{S9}$$

as stated in Eq. (3) in the main text.

The above argument can be extended to any symmetric finite-rank perturbation matrix $\tilde{\boldsymbol{R}}_n$ with eigenvalues $\theta_i$ [5]. Such a matrix can always be written in terms of an $M\times n$ matrix $\boldsymbol{U}_n$ with orthonormal columns and a diagonal matrix $\boldsymbol{\Theta}=\mathrm{diag}(\theta_i)$, as $\tilde{\boldsymbol{R}}_n=\boldsymbol{U}_n\boldsymbol{\Theta}\boldsymbol{U}_n^{\mathsf{T}}$. Then $\lambda$ will be an eigenvalue of $\tilde{\boldsymbol{X}}+\tilde{\boldsymbol{R}}_n$ and not of $\tilde{\boldsymbol{X}}$ if

$$\boldsymbol{I}_n-\boldsymbol{U}_n^{\mathsf{T}}(\lambda \boldsymbol{I}-\tilde{\boldsymbol{X}})^{-1}\boldsymbol{U}_n\boldsymbol{\Theta} \tag{S10}$$

has a zero eigenvalue, where $\boldsymbol{I}_n$ is the $n\times n$ identity matrix. If the columns of $\boldsymbol{U}_n$ are again in random orientations, $\boldsymbol{U}_n^{\mathsf{T}}(\lambda \boldsymbol{I}-\tilde{\boldsymbol{X}})^{-1}\boldsymbol{U}_n$ can be replaced by $(\boldsymbol{I}_n/M)\mathrm{Tr}(\lambda \boldsymbol{I}-\tilde{\boldsymbol{X}})^{-1}=G_{\tilde{X}}(\lambda)\boldsymbol{I}_n$ for $M\to\infty$. The condition for (S10) to have a zero eigenvalue then reduces to the analog of (S6) for each $\theta_i$, and the spinodal equation (S9) follows with $\theta=\min(\theta_i)$. This can be seen by realizing that $G_{\tilde{X}}(\lambda)$ in (S6) is monotonically decreasing outside the spectrum of $\tilde{\boldsymbol{X}}$, meaning the outlier relevant to the spinodal ($\lambda=0$) is the one where $\theta_i^{-1}$ is closest to zero, i.e. where $|\theta_i|$ is largest. Given that $\theta_i$ has to be negative to create an outlier to the left of the bulk of $\tilde{\boldsymbol{X}}$, one concludes that the $\theta_i$ relevant to the spinodal is $\theta=\min(\theta_i)$.

## II. Bulk Regime

If an outlier does not exist to the left of the bulk, then the lowest eigenvalue of $\tilde{\boldsymbol{H}}$ is given by the lower edge of the bulk, i.e. of the spectrum of $\tilde{\boldsymbol{D}}+\tilde{s}\tilde{\boldsymbol{\eta}}$. We follow [6] and, defining $g(z)=G_{\tilde{D}+\tilde{s}\tilde{\eta}}(z)-z/\tilde{s}^2$, recast the Pastur relation (S3) as

$$z=-\tilde{s}^2[g-G_{\tilde{D}}(-\tilde{s}^2g)]\equiv F(g). \tag{S11}$$

The general formula

$$p(\lambda)=\frac{1}{\pi}\lim_{\epsilon\to0^+}\mathrm{Im}[G_X(\lambda-i\epsilon)] \tag{S12}$$

for inverting (S1) shows that $g(z)$ will be real for $z$ outside the spectrum of $\tilde{\boldsymbol{D}}+\tilde{s}\tilde{\boldsymbol{\eta}}$ and otherwise complex. Conversely, as $g$ varies across real values, the only real values of $z = F(g)$ that will result must lie *outside* the spectrum. Therefore, the edges of the spectrum are determined by the minima and maxima of $F(g)$ for real $g$; these delimit the "forbidden" range of $z$ from above and below. Here, we focus on the lower edge, i.e. the maximum of $F(g)$ on its lower branch, as it is the one determining the lowest eigenvalue.

Since $G_{\tilde{D}}(-\tilde{s}^2 g)$ for real $g$ can have complex values only when $-\tilde{s}^2 g$ lies between the smallest and largest eigenvalue of $\tilde{\boldsymbol{D}}$, i.e. when $-T/(\tilde{s}^2\rho y_{\min}) < g < -T/(\tilde{s}^2\rho y_{\max})$, it follows that $F(g)$ must be real for $g > -T/(\tilde{s}^2\rho y_{\max})$ (see Fig. S1). Then, as shown in [6] there are two possibilities for its maximum and hence the lower spectral edge. If $F(g)$ has a maximum $g^*$ for $g > -T/(\tilde{s}^2\rho y_{\max})$, then the diagonal matrix $\tilde{\boldsymbol{D}}$ is qualitatively similar to an identity matrix as far its effect on the edges of the spectrum is concerned, meaning the eigenvalues of the Wigner matrix $\tilde{s}\tilde{\boldsymbol{\eta}}$ are essentially only shifted and the eigenvectors remain delocalized [6, 7]. On the other hand, if $F(g)$ has no maximum for $g > -T/(\tilde{s}^2\rho y_{\max})$, then $g^* = -T/(\tilde{s}^2\rho y_{\max})$ and the spectral edge is determined by the diagonal matrix $\tilde{\boldsymbol{D}}$. A transition from the Wigner dominated to the diagonal dominated case happens when a stationary point occurs at $g^* = -T/(\tilde{s}^2\rho y_{\max})$, i.e. $F'(-T/\tilde{s}^2\rho y_{\max}) = 0$, which yields Eq. (5) in the main text.

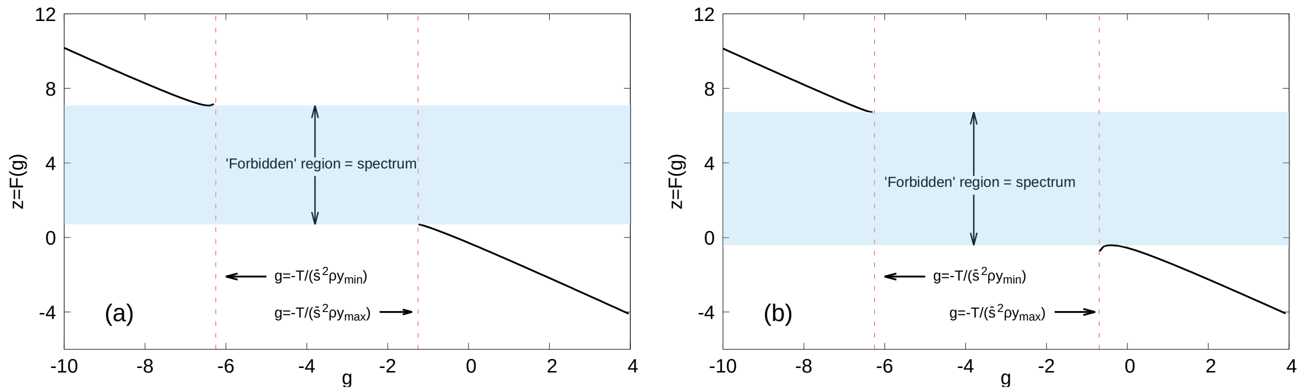


FIG. S1. Illustration of $F(g)$ in the case of a Beta distribution of relative densities. The "forbidden" region on the $y$-axis for real $g$ corresponds to the bulk of the spectrum of $\tilde{\boldsymbol{H}}$. In (a), for the parameters used (chosen for illustration purposes only), $F(g)$ has no maximum to the right of $-T/(\tilde{s}^2\rho y_{\max})$, represented by the vertical dashed line, meaning the composition dominates the lower edge of the spectrum, which is given by $F(-T/(\tilde{s}^2\rho y_{\max}))$. In (b) the Wigner matrix dominates and $F(g)$ has a maximum for $g > -T/(\tilde{s}^2\rho y_{\max})$.

The condition that we are at the spinodal is that the lower spectral edge is at $z = 0$, hence $F(g^*) = 0$, or $g^* = G_{\tilde{D}}(-\tilde{s}^2 g^*)$. Following the same approach as in the outlier regime, this condition can be recast as

$$\psi_y(-\rho\tilde{s}^2 g^*/T) = (\tilde{s}g^*)^2 \tag{S13}$$

with $g^*$ determined as discussed above.

By comparing the spinodal equation in the outlier and bulk regimes we see that the two solutions coincide when $g^* = \theta^{-1}$, giving a numerically convenient way to evaluate the outlier-bulk transition. This can also be seen by noticing that the lowest edge of the bulk $\lambda_-$ and the outlier coincide at the spinodal, i.e. $\lambda_- = 0$, whenever (see S6) $g^* = G_{\tilde{D}+\tilde{s}\tilde{\eta}}(\lambda_- = 0) = \theta^{-1}$.

## 2. FINITE SIZE EFFECTS

The first source of finite size effects in our equations is the possible $M$-dependence of the perturbation matrix $\boldsymbol{R}_n$ and in particular its eigenvalues and eigenvectors. For $n = 1$ this is not an issue as there is a single $M$-independent eigenvalue $\theta = T/\rho - b$. For $n > 1$ as in the example in Sec. 5 (and corresponding results in the main text), the eigenvalues do have an $M$-dependence (see e.g. the definition of $y_2$) and we retain this when comparing with numerical evaluations of the spinodal from samples of the Hessian. This is not a fully controlled procedure as we ignore corrections to the $M \to \infty$ predictions of free probability that could be of the same order. The effects of the corrections can be seen in the eigenvector projections in Figs. 2 and 3, as well as the smooth transition from condensation to composition-dependent demixing in the spinodal for $y_1 = 20$ in Fig. 2. Without corrections, i.e. in

the true $M \to \infty$ limit, sharp transitions would appear as given in the analytical expressions throughout this work; the correction terms clearly lead to better agreement with the numerical results for finite $M$.

Another source of finite size effects lies in the step where we derived the spinodal equation by assuming that the lowest eigenvalue in the bulk sits exactly at the edge $\lambda_0$ of the $M \to \infty$ distribution. This is clearly true in the large $M$ limit, while for a finite number of mixture components Sear and Cuesta [8] proposed to estimate a corrected eigenvalue $\lambda(M)$ using extreme value theory, with the criterion that the cumulative probability in the spectrum should be $1/M$:

$$\int_{\lambda_0}^{\lambda(M)} P(\lambda) d\lambda = \frac{1}{M}. \tag{S14}$$

In the Beta distribution case, for $T > T^*$, this would lead to corrections of order $O(M^{-1/(t+1)})$ in the location of the lowest eigenvalue as well as finite-size corrections to the eigenvector overlaps as pointed out in [9]. As $\lambda(M)$ always lies above $\lambda_0$, a spinodal instability will be reached later coming from high temperatures so that we expect the spinodal curves for finite $M$ in the bulk regime to lie slightly below the ones predicted in the limit $M \to \infty$.

## 3. EIGENVECTOR OVERLAP

Here we outline how to obtain equation (4) for the overlap of the instability direction $\boldsymbol{v}$ with the leading (lowest eigenvalue) eigenvector of $\boldsymbol{R}_n$. We discuss directly the more general result for rank-$n$ perturbation matrices.

For a finite rank perturbation $\boldsymbol{R}_n$ of a large random matrix, i.e. $\tilde{\boldsymbol{H}} = \boldsymbol{R}_n + \tilde{\boldsymbol{D}} + \tilde{s}\tilde{\boldsymbol{\eta}}$, let $\boldsymbol{w}_i$, $i = 1 \dots n$, be the eigenvectors of $\boldsymbol{R}_n$ corresponding to the nonzero eigenvalues $\theta_i$. We first identify the direction of the eigenvector $\boldsymbol{v}$ corresponding to the lowest eigenvalue $\lambda_{\min}$ of $\tilde{\boldsymbol{H}}$ using the resolvent matrix $\boldsymbol{G}_{\tilde{H}}(\lambda)$. Decomposing $\tilde{\boldsymbol{H}}$ in terms of its eigenvalues $\lambda_a$ and eigenvectors $\boldsymbol{v}_a$ gives

$$\boldsymbol{G}_{\tilde{H}}(\lambda) = (\lambda \boldsymbol{I} - \tilde{\boldsymbol{H}})^{-1} = \sum_a \frac{\boldsymbol{v}_a \boldsymbol{v}_a^\top}{\lambda - \lambda_a} = \frac{\boldsymbol{v}\boldsymbol{v}^\top}{\lambda - \lambda_{\min}} + \dots \tag{S15}$$

The term for $\lambda_a = \lambda_{\min}$ that we have isolated on the right gives the only divergent contribution for $\lambda \to \lambda_{\min}$ so that

$$\lim_{\lambda \to \lambda_{\min}} (\lambda - \lambda_{\min}) \boldsymbol{G}_{\tilde{H}}(\lambda) = \boldsymbol{v}\boldsymbol{v}^\top. \tag{S16}$$

The overlap between $\boldsymbol{v}$ and a chosen eigenvector $\boldsymbol{w}_\theta \in \{\boldsymbol{w}_i\}$ of $\boldsymbol{R}_n$ with eigenvalue $\theta$ is then

$$|\boldsymbol{v}^\top \boldsymbol{w}_\theta|^2 = \lim_{\lambda \to \lambda_{\min}} (\lambda - \lambda_{\min}) \boldsymbol{w}_\theta^\top \boldsymbol{G}_{\tilde{H}}(\lambda) \boldsymbol{w}_\theta. \tag{S17}$$

Writing, as before, $\boldsymbol{R}_n = \boldsymbol{U}_n \Theta \boldsymbol{U}_n^\top$ one can use the Woodbury identity to obtain

$$\boldsymbol{G}_{\tilde{H}}(\lambda) = \boldsymbol{G}_{\tilde{\boldsymbol{D}}+\tilde{s}\tilde{\boldsymbol{\eta}}} + \boldsymbol{G}_{\tilde{\boldsymbol{D}}+\tilde{s}\tilde{\boldsymbol{\eta}}} \boldsymbol{U}_n \left( \Theta^{-1} - \boldsymbol{U}_n^\top \boldsymbol{G}_{\tilde{\boldsymbol{D}}+\tilde{s}\tilde{\boldsymbol{\eta}}} \boldsymbol{U}_n \right)^{-1} \boldsymbol{U}_n^\top \boldsymbol{G}_{\tilde{\boldsymbol{D}}+\tilde{s}\tilde{\boldsymbol{\eta}}}. \tag{S18}$$

The condition that the eigenvectors of $\boldsymbol{R}_n$, i.e. the columns of $\boldsymbol{U}_n$ lie in generic positions with respect to those of $\tilde{\boldsymbol{D}} + \tilde{s}\tilde{\boldsymbol{\eta}}$ results in

$$\boldsymbol{U}_n^\top \boldsymbol{G}_{\tilde{\boldsymbol{D}}+\tilde{s}\tilde{\boldsymbol{\eta}}} \boldsymbol{U}_n \simeq G_{\tilde{\boldsymbol{D}}+\tilde{s}\tilde{\boldsymbol{\eta}}} \boldsymbol{I}_n \qquad \text{and} \qquad \boldsymbol{w}_\theta^\top \boldsymbol{G}_{\tilde{\boldsymbol{D}}+\tilde{s}\tilde{\boldsymbol{\eta}}} \boldsymbol{w}_\theta \simeq G_{\tilde{\boldsymbol{D}}+\tilde{s}\tilde{\boldsymbol{\eta}}} \tag{S19}$$

where $G_{\tilde{\boldsymbol{D}}+\tilde{s}\tilde{\boldsymbol{\eta}}}$ is the normalized trace of $\boldsymbol{G}_{\tilde{\boldsymbol{D}}+\tilde{s}\tilde{\boldsymbol{\eta}}}$ as usual. The expression on the r.h.s. of (S17) then simplifies to

$$\boldsymbol{w}_\theta^\top \boldsymbol{G}_{\tilde{H}}(\lambda) \boldsymbol{w}_\theta = G_{\tilde{\boldsymbol{D}}+\tilde{s}\tilde{\boldsymbol{\eta}}} + \boldsymbol{w}_\theta^\top \boldsymbol{G}_{\tilde{\boldsymbol{D}}+\tilde{s}\tilde{\boldsymbol{\eta}}} \boldsymbol{U}_n \left( \Theta^{-1} - G_{\tilde{\boldsymbol{D}}+\tilde{s}\tilde{\boldsymbol{\eta}}} \boldsymbol{I}_n \right)^{-1} \boldsymbol{U}_n^\top \boldsymbol{G}_{\tilde{\boldsymbol{D}}+\tilde{s}\tilde{\boldsymbol{\eta}}} \boldsymbol{w}_\theta. \tag{S20}$$

Since the term in brackets is a diagonal matrix and $\boldsymbol{U}_n$ has the $\boldsymbol{w}_i$ as columns, one can equivalently write

$$\boldsymbol{w}_\theta^\top \boldsymbol{G}_{\tilde{H}}(\lambda) \boldsymbol{w}_\theta = G_{\tilde{\boldsymbol{D}}+\tilde{s}\tilde{\boldsymbol{\eta}}} + \sum_i \left( \boldsymbol{w}_\theta^\top \boldsymbol{G}_{\tilde{\boldsymbol{D}}+\tilde{s}\tilde{\boldsymbol{\eta}}} \boldsymbol{w}_i \right)^2 \left( \theta_i^{-1} - G_{\tilde{\boldsymbol{D}}+\tilde{s}\tilde{\boldsymbol{\eta}}} \right)^{-1} = G_{\tilde{\boldsymbol{D}}+\tilde{s}\tilde{\boldsymbol{\eta}}} + \frac{\theta G^2_{\tilde{\boldsymbol{D}}+\tilde{s}\tilde{\boldsymbol{\eta}}}}{1 - \theta G_{\tilde{\boldsymbol{D}}+\tilde{s}\tilde{\boldsymbol{\eta}}}}, \tag{S21}$$

where $\boldsymbol{w}_\theta^\top \boldsymbol{G}_{\tilde{\boldsymbol{D}}+\tilde{s}\tilde{\boldsymbol{\eta}}} \boldsymbol{w}_i = G_{\tilde{\boldsymbol{D}}+\tilde{s}\tilde{\boldsymbol{\eta}}} \delta_{i\theta}$ by (S19). Finally, inserting (S21) into (S17) yields

$$|\boldsymbol{v}^\top \boldsymbol{w}_\theta|^2 = \lim_{\lambda \to \lambda_{\min}} (\lambda - \lambda_{\min}) \frac{\theta G^2_{\tilde{\boldsymbol{D}}+\tilde{s}\tilde{\boldsymbol{\eta}}}(\lambda)}{1 - \theta G_{\tilde{\boldsymbol{D}}+\tilde{s}\tilde{\boldsymbol{\eta}}}(\lambda)}. \tag{S22}$$

The remaining limit in (S22) can be evaluated using L'Hôpital's rule and the condition (S6) for $\lambda_{\min}$. Using that condition again to simplify the numerator results in

$$|\boldsymbol{v}^\top \boldsymbol{w}_\theta|^2 = -\frac{G^2_{\tilde{D}+\tilde{s}\tilde{\eta}}(\lambda_{\min})}{G'_{\tilde{D}+\tilde{s}\tilde{\eta}}(\lambda_{\min})} = -\frac{1}{\theta^2 G'_{\tilde{D}+\tilde{s}\tilde{\eta}}(\lambda_{\min})} \tag{S23}$$

Using the Pastur relation (S3) we can further express $G'_{\tilde{D}+\tilde{s}\tilde{\eta}}(\lambda_{\min})$ in terms of $G'_{\tilde{D}}(\lambda_{\min})$ as

$$\frac{1}{G'_{\tilde{D}+\tilde{s}\tilde{\eta}}(\lambda_{\min})} = \tilde{s}^2 + \frac{1}{G'_{\tilde{D}}(\lambda_{\min} - \tilde{s}^2 G_{\tilde{D}+\tilde{s}\tilde{\eta}}(\lambda_{\min}))}. \tag{S24}$$

Evaluating this expression at the spinodal, that is at $\lambda_{\min} = K_{\tilde{D}+\tilde{s}\tilde{\eta}}(\theta^{-1}) = 0$ and inserting the resulting expression into (S23) we obtain the expression (4) found in the main text.

## 4. FREENESS CONDITION

As discussed in the main text and the previous sections in the SM, in order to allow us to apply tools from free probability theory, the matrices $\tilde{\boldsymbol{R}}_1$, $\tilde{\boldsymbol{D}}$ and $\tilde{s}\tilde{\boldsymbol{\eta}}$ must satisfy some key assumptions. To keep things general, we drop the rank one restriction and investigate these assumptions for any finite rank matrix $\tilde{\boldsymbol{R}}_n$.

First, we used the free sum rule between the matrices $\tilde{\boldsymbol{D}}$ and $\tilde{s}\tilde{\boldsymbol{\eta}}$. Given that two matrices are free if their eigenvectors lie in generic positions with respect to each other or, equivalently, the overlap between their eigenvectors is of $O(M^{-1/2})$, the freeness between $\tilde{\boldsymbol{D}}$ and $\tilde{s}\tilde{\boldsymbol{\eta}}$ follows from the eigenvectors of the latter being uniformly distributed on the unit sphere while those of the former, namely the Cartesian unit vectors, are fully localized on a single entry. This justifies our derivations in the bulk regime.

Second, when deriving the position of the outlier, we took the matrix $\tilde{\boldsymbol{X}} = \tilde{\boldsymbol{D}} + \tilde{s}\tilde{\boldsymbol{\eta}}$ as diagonal after an appropriate basis change. Such a change of basis preserves the eigenvalue distribution of $\tilde{\boldsymbol{H}}$, but results in a corresponding rotation of the eigenvectors of $\tilde{\boldsymbol{R}}_n$. We assumed in our derivations that after this rotation, the eigenvectors of $\tilde{\boldsymbol{R}}_n$ are in generic position. This is clearly true in the Wigner dominated regime, i.e. when $\tilde{s}\tilde{\boldsymbol{\eta}}$ dominates the sum defining $\tilde{\boldsymbol{X}}$, because the eigenvectors of $\tilde{s}\tilde{\boldsymbol{\eta}}$ are randomly distributed on the unit sphere so that the basis change performs a random rotation of the eigenvectors of $\tilde{\boldsymbol{R}}_n$.

Potential freeness violations could therefore occur only in the opposite limit, where $\tilde{\boldsymbol{X}}$ is dominated by $\tilde{\boldsymbol{D}}$. The latter has as eigenvectors the Cartesian unit vectors so no basis change is then necessary. As a consequence, freeness requires simply that the eigenvectors of $\tilde{\boldsymbol{R}}_n$ are extended, with components of $O(M^{-1/2})$, rather than being localized, i.e. concentrated onto a few species. In the rank one case as presented in the main text, the eigenvector of $\tilde{\boldsymbol{R}}_1$ is uniform, with components $\hat{u}_\alpha = M^{-1/2}$, so this condition for freeness is evidently satisfied. For $n > 1$, including systematic interactions of the form $-\boldsymbol{\sigma}\boldsymbol{\sigma}^\top$ in $\tilde{\boldsymbol{R}}_n$ preserves the freeness condition if all components $\sigma_\alpha$ of $\boldsymbol{\sigma}$ are of same order, e.g. within some constant factor of each other. An exception would be a case where one component $\sigma_\alpha$ dominates significantly over the others, e.g. $\sigma_1 = 1$ and all other $\sigma_\alpha = 0$. In summary, as long as $\tilde{\boldsymbol{R}}_n$ does not have any localized eigenvectors, the use of free probability theory in our derivations is fully justified.

## 5. ONE DOMINANT SPECIES

In this section we derive the explicit predictions of our approach for the example of one dominant species discussed in the main text.

This is a case when the distribution of the $y_\alpha$ contains an outlier so that the "bulk" spectrum of $\tilde{\boldsymbol{D}} + \tilde{s}\tilde{\boldsymbol{\eta}}$ can contain an outlier itself. Nonetheless, as the discussion below will show, instabilities caused by such "bulk outliers" conform to the classification used in the main text: they are caused by the bulk and are therefore of demixing type.

We exploit the extension of the rank-one perturbation results to general finite-rank perturbations by rewriting the Hessian matrix as $\boldsymbol{H} = \boldsymbol{R}_1 + \Delta \boldsymbol{e}_1 \boldsymbol{e}_1^\top + \boldsymbol{D}_2 + s\boldsymbol{\eta}$, where $\Delta = T(y_2 - y_1)/(\bar{\rho} y_2 y_1)$, $\boldsymbol{e}_1 = (1, 0, 0, \ldots, 0)^\top$ and $\boldsymbol{D}_2 = T/(\bar{\rho} y_2)\boldsymbol{I}$. This is an equivalent statement of our stability problem since $\boldsymbol{D} = \Delta \boldsymbol{e}_1 \boldsymbol{e}_1^\top + \boldsymbol{D}_2$, but it allows us to treat $\boldsymbol{R}_1 + \Delta \boldsymbol{e}_1 \boldsymbol{e}_1^\top$ as a rank-two perturbation of $\boldsymbol{D}_2 + s\boldsymbol{\eta}$. As previously pointed out, we consider the rescaled Hessian $\tilde{\boldsymbol{H}} = \boldsymbol{H}/M$ and similarly define $\tilde{\Delta} = \Delta/M = T(y_2 - y_1)/(\rho y_2 y_1)$, which for $M \to \infty$ and hence $y_2 = (M - y_1)/(M - 1) \to 1$ simplifies to $\tilde{\Delta} = -(T/\rho)(1 - y_1^{-1})$.

In order to find the spinodal equation (3) in the outlier regime one needs to first solve the deterministic eigensystem to find the lowest eigenvalue $\theta$ of $M^{-1}(\boldsymbol{R}_1 + \Delta \boldsymbol{e}_1 \boldsymbol{e}_1^\top)$ with corresponding eigenvector $\boldsymbol{w}_\theta$. In the large $M$ limit we find

$\theta = \min\{T/\rho_0 - b, \tilde{\Delta}\}$. (For numerical evaluation of the theory we retain the finite-$M$ versions of $y_2$ and $\theta$ as explained above.) At the point where $\theta$ changes from one "branch" of the minimum to the other as the density is increased, there is a discontinuous jump of the eigenvector $\boldsymbol{w}_\theta$ from $\hat{\boldsymbol{u}}$ to $\boldsymbol{e}_1$. Corresponding to this we have a transition in the spinodal equation (3) from condensation to composition-driven demixing. The consequences of this transition from the C to the CD eigenvector can be seen in Fig. 2 in the main text.

For the instability direction, the eigenvector overlap can be obtained by direct analogy with the uniform composition case because the deviation of $\boldsymbol{D}$ from $\boldsymbol{D}_2$ is already covered explicitly in the rank-two perturbation $\boldsymbol{R}_1 + \Delta \boldsymbol{e}_1 \boldsymbol{e}_1^\mathsf{T}$. The results reads $|\boldsymbol{v}^\mathsf{T} \boldsymbol{w}_\theta|^2 = 1 - \tilde{s}^2/\theta^2$, where $\boldsymbol{w}_\theta$ is either $\hat{\boldsymbol{u}}$ or $\boldsymbol{e}_1$ as discussed above, while the projection onto the orthogonal direction within the space spanned by $\boldsymbol{e}_1$ and $\hat{\boldsymbol{u}}$ is zero [5].

## 6. TWO GROUPS OF SPECIES

In this section we discuss the spinodal instability behaviour for a system with the distribution of relative densities

$$p(y_\alpha) = a\delta(y_\alpha - y_1) + (1-a)\delta(y_\alpha - y_2) \tag{S25}$$

This corresponds to having two groups of species, one group of size $aM$ with relative density $y_1$ and another of size $(1-a)M$ with relative density $y_2 < y_1$. The three parameters are linked by the constraint $\langle y \rangle = ay_1 + (1-a)y_2 = 1$. We will show that this composition gives similar predictions to the case of one dominant species discussed above, and that it recovers this case when $a \sim 1/M \to 0$.

If $y_1$ and $y_2$ are sufficiently different, the bulk of the spectrum will have two disconnected pieces, each containing a fraction $a$ and $1-a$ of the eigenvalues. For $a \to 0$ the piece of size $a$ extrapolates to the "bulk outlier" we observed in the case of one dominant species. The spinodal equation (3) in the main text yields, for the composition (S25)

$$-\beta\rho \left[ \frac{ay_1}{1 + \beta\rho\tilde{s}^2 z y_1} + \frac{(1-a)y_2}{1+\beta\rho\tilde{s}^2 z y_2} \right] = z \tag{S26}$$

This can easily be solved solved in the outlier regime, where $z = (-b + T/\rho_0)^{-1}$. In the bulk regime, one solves instead $F'(g^*) = 0$ or, equivalently,

$$\frac{ay_1^2}{(T/(\tilde{s}^2\rho g^*) + y_1)^2} + \frac{(1-a)y_2^2}{(T/(\tilde{s}^2\rho g^*) + y_2)^2} = (\tilde{s} g^*)^2 \tag{S27}$$

for $g^*$ and uses $z = g^*$.

We show in Fig. S2 the resulting spinodal curves for a range of values of $a$, with $y_1$ fixed and adjusting $y_2$ to keep $\langle y \rangle$ fixed. We observe that, as expected, the predictions for the single dominant species case are recovered in the limit $a \to 0$. Note that the predictions for a single dominant species that we compare to are evaluated with some finite-$M$ corrections included as explained in Sec. (2). One could attempt to incorporate such also in the case of two groups of species by setting $a = 1/M$. As these corrections are not systematic, however, and ignore finite-$M$ corrections to the free probability framework itself, it turns out that $a \to 0$ gives a better match to the data for one dominant species (see Fig. S2).

By analyzing the nature of the instability via the leading eigenvector composition, we find that for $a \sim O(1)$ the projection of $\boldsymbol{v}$ onto $\boldsymbol{e}_1$ – or indeed any other single species – goes to zero for large $M$. One can show, on the other hand, that the instability direction $\boldsymbol{v}$ will, in the demixing regime, have a nonzero projection within the subspace spanned by the $aM$ Cartesian unit vectors of the species with the higher density $y_1$. The demixing would then be led by these $aM$ dominant species.

## 7. MODEL EXTENSIONS

In the main text we briefly mentioned possible extensions of the model. We now expand on these extensions and show how they fit into our framework.

In Ref. [10], a deterministic additive interaction model has been considered where each component is characterized by a finite number of features encoded in the vectors $\boldsymbol{\sigma}_i$ such that the virial coefficients are $\hat{\boldsymbol{\epsilon}} = \sum_i \boldsymbol{\sigma}_i \boldsymbol{\sigma}_i^\mathsf{T}$; $i$ here labels the different features. Notice that this model does not contain any random interaction. Using the framework developed here, one could readily study an extended model that includes random interactions, by considering $\boldsymbol{\epsilon} = \hat{\boldsymbol{\epsilon}} - b\boldsymbol{u}\boldsymbol{u}^\mathsf{T} + s\boldsymbol{\eta}$, with $\hat{\boldsymbol{\epsilon}} - b\boldsymbol{u}\boldsymbol{u}^\mathsf{T}$ then a finite-rank perturbation to the Wigner matrix $s\boldsymbol{\eta}$.

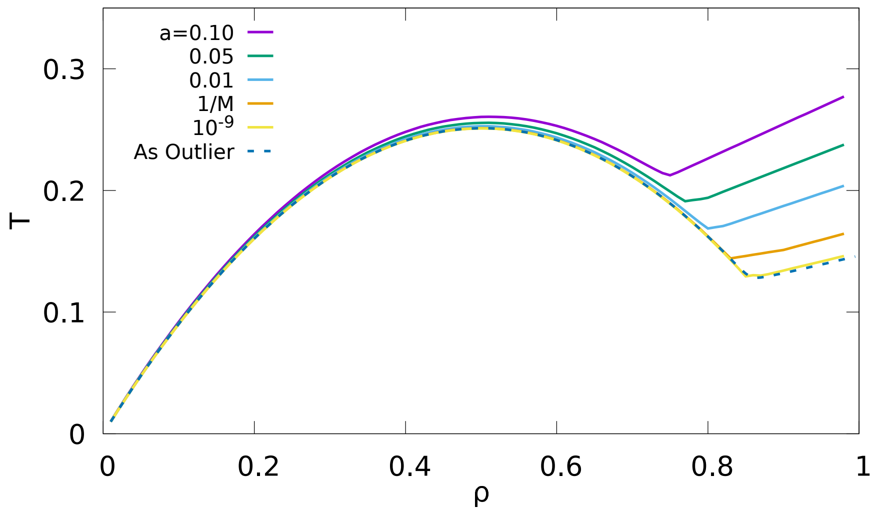


FIG. S2. Two groups of species. Spinodal lines obtained numerically for different values of $a$ as it approaches 0, at fixed relative density $y_1 = 10$. The dashed line gives the predictions for a single dominant species, where $y_1$ is treated as an outlier, in a mixture of size $M = 500$. The results for two groups of species agree in the limit $a \to 0$.

Another recent model [11] considers a mixture of many components split into $F$ families such that the average interaction between families $f_i$ and $f_j$ is $\mu_{ij}$ and the variance of the random part is $S_{ij}^2$. The virial coefficients of this model are written as $\boldsymbol{\epsilon} = \boldsymbol{\mu} + \boldsymbol{S} * \boldsymbol{\eta}$, where the star product denotes the element-wise multiplication and both $\boldsymbol{\mu}$ and $\boldsymbol{S}$ are $M \times M$ block-matrices consisting of $F \times F$ blocks and with constant values within each block. Due to the family construction, the matrix $\boldsymbol{\epsilon}$ also has a block structure. Assuming a *uniform composition* and ignoring the entropic contribution of the solvent, the authors of Ref. [11] obtained the spinodal line and the composition of the leading instability. The connection to our treatment is that, since the matrix $\boldsymbol{\mu}$ is symmetric and has a block structure with $F$ families, its rank is no larger than $F$ and it can therefore always be written in a form that makes this explicit, $\boldsymbol{\mu} \equiv \boldsymbol{R}_F = \sum_{i=1}^{F} \boldsymbol{\sigma}_i \boldsymbol{\sigma}_i^{\mathsf{T}}$. As long as we take the matrix $\boldsymbol{S}$ to be constant, the treatment of the model of Ref. [11] can therefore be directly extended to any composition using our finite-rank framework.

The case of non-constant $\boldsymbol{S}$ can also be treated in our framework if we assume a rank one structure $\boldsymbol{S} = \boldsymbol{s}\boldsymbol{s}^{\mathsf{T}}$. The element-wise product $\boldsymbol{S} * \boldsymbol{\eta}$ can then be written as $\boldsymbol{D}_s^{1/2} \boldsymbol{\eta} \boldsymbol{D}_s^{1/2}$, where $\boldsymbol{D}_s = \mathrm{diag}(\boldsymbol{s})$. Free probability now gives a route to computing the spectrum of the resulting matrix, by using the free product rule $S_{A^{1/2}BA^{1/2}}(z) = S_A(z) S_B(z)$ where the $S$-transform is defined by $S(z) = \frac{1+z}{z}\psi^{-1}(z)$ and $S_\eta = \pm\frac{1}{\sqrt{z}}$. The additive finite-rank perturbation $\boldsymbol{\mu}$ can finally be included via the free sum rule.

---


[1] G. Akemann, J. Baik, and P. Di Francesco, *The Oxford handbook of random matrix theory* (Oxford University Press, 2011).
[2] Z. Burda, Journal of Physics: Conference Series **473**, 12002 (2013).
[3] Z. Bai, B. Miao, and J. Tsay, Journal of Theoretical Probability **12**, 301 (1999).
[4] L. A. Pastur, Theoretical and Mathematical Physics **10**, 67 (1972).
[5] F. Benaych-Georges and R. R. Nadakuditi, Advances in Mathematics **227**, 494 (2011), arXiv:0910.2120.
[6] E. Bouchbinder, E. Lerner, C. Rainone, P. Urbani, and F. Zamponi, Physical Review B **103**, 1 (2021), arXiv:2012.11558.
[7] C. F. Lee and J. D. Wurtz, "Novel physics arising from phase transitions in biology," (2018), arXiv:1809.11117.
[8] R. P. Sear and J. A. Cuesta, Physical Review Letters **91**, 1 (2003), arXiv:0307326 [cond-mat].
[9] J. O. Lee and K. Schnelli, Probability Theory and Related Fields **164**, 165 (2016), arXiv:1310.7057.
[10] I. R. Graf and B. B. Machta, Physical Review Research **4**, 033144 (2022).
[11] G. Carugno, I. Neri, and P. Vivo, Physical Biology (2022).
